# Supplementary material for: Simulating 2D topological quantum phase transitions on a digital quantum computer
Source: arXiv:2312.05079 source file (2024-09-28)
Supplement: Supplementary file 1 [file sm_pullthrough.pdf]

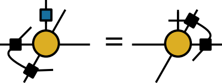

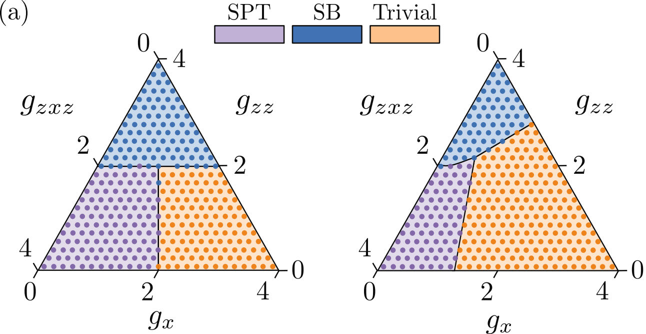
(a)
SPT
SB
Trivial
$g_{zxz}$
$g_{zz}$
$g_x$
0
4
2
2
4
0
0
2
4
$g_{zxz}$
$g_{zz}$
$g_x$
0
4
2
2
4
0
0
2
4

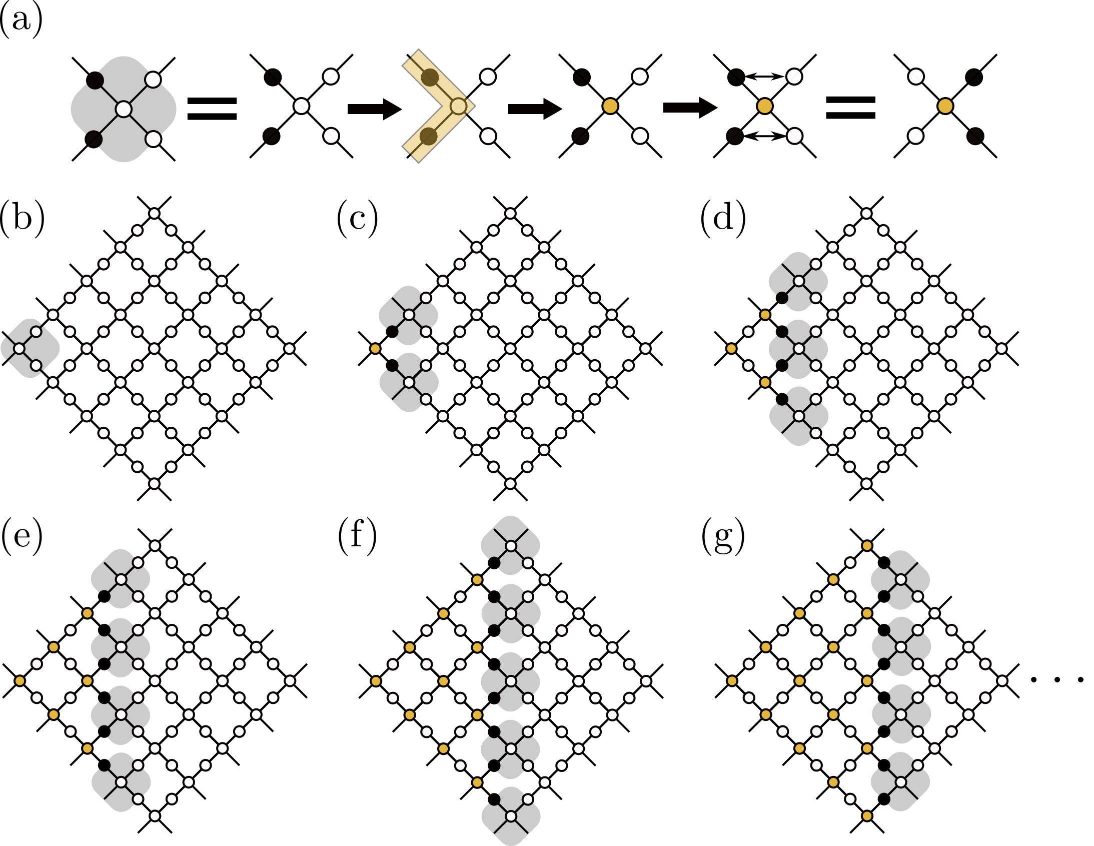
(a)
(b)
(c)
(d)
(e)
(f)
(g)

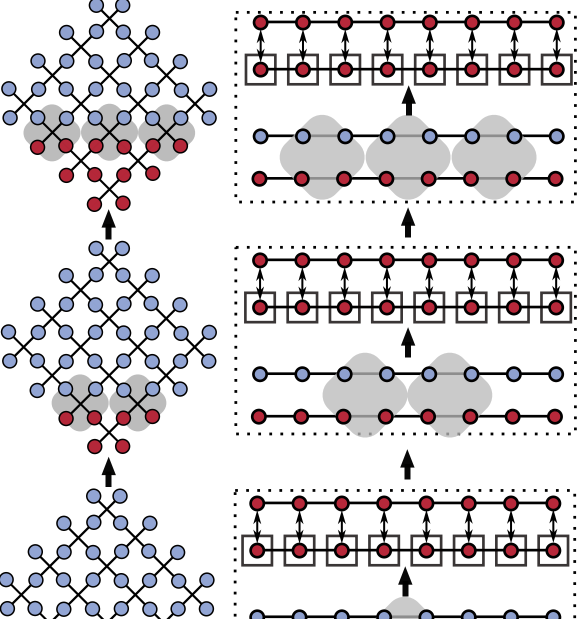

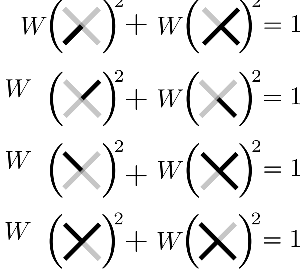

W
W
W
W


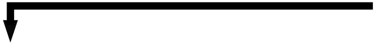

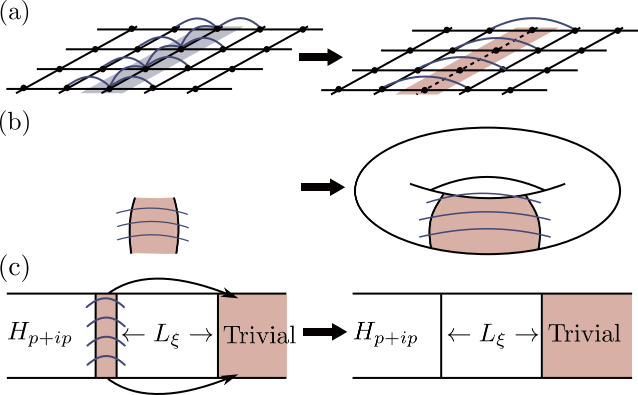

(a)
(b)
(c)
$H_{p+ip}$
$\leftarrow L_\xi \rightarrow$
Trivial
$H_{p+ip}$
$\leftarrow L_\xi \rightarrow$
Trivial
