# Supplementary material for: Simulating 2D topological quantum phase transitions on a digital quantum computer
Source: arXiv:2312.05079 source file (2024-09-28)

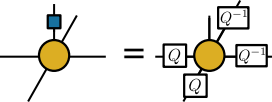

(a)

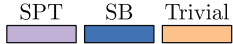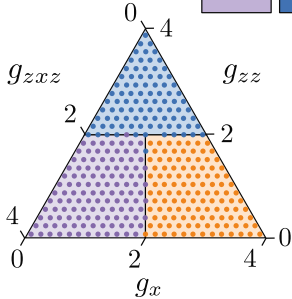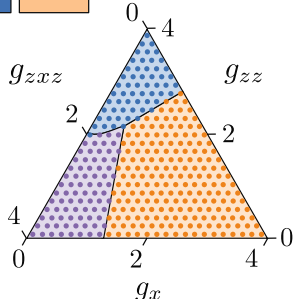

(a)

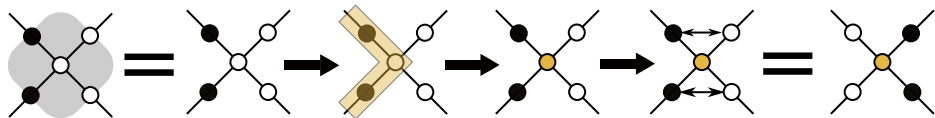

(b)

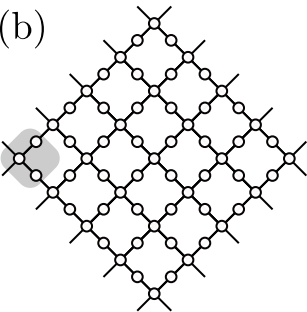

(c)

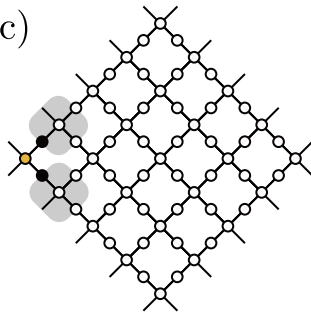

(d)

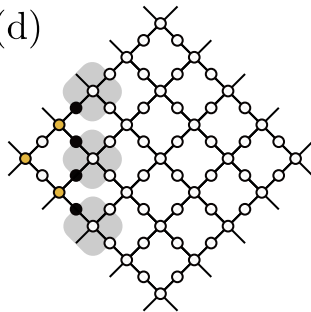

(e)

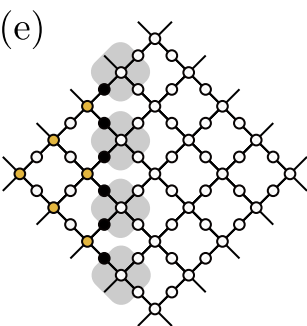

(f)

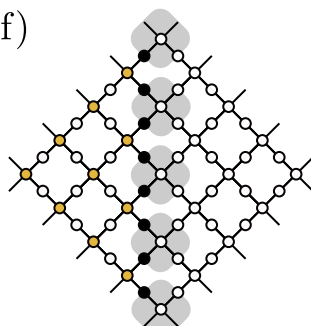

(g)

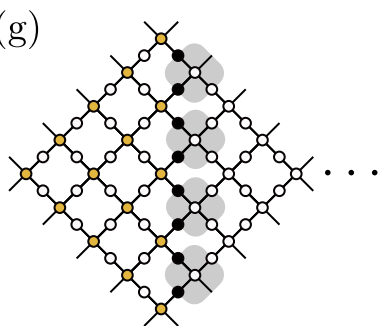



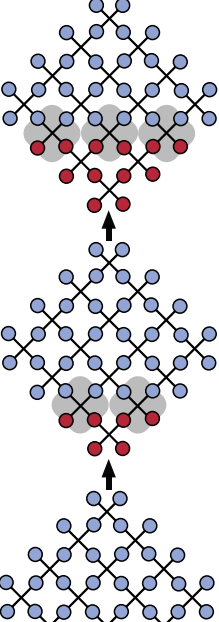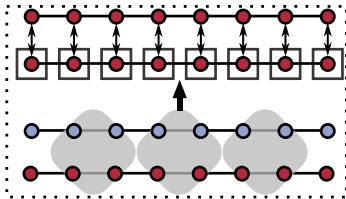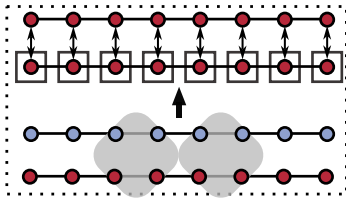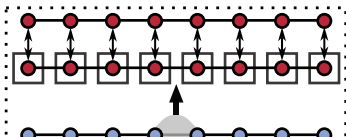

$$W\left(\begin{array}{c} \text{X} \\ \text{X} \end{array}\right)^2 + W\left(\begin{array}{c} \text{X} \\ \text{X} \end{array}\right)^2 = 1$$

$$W\left(\begin{array}{c} \text{X} \\ \text{X} \end{array}\right)^2 + W\left(\begin{array}{c} \text{X} \\ \text{X} \end{array}\right)^2 = 1$$

$$W\left(\begin{array}{c} \text{X} \\ \text{X} \end{array}\right)^2 + W\left(\begin{array}{c} \text{X} \\ \text{X} \end{array}\right)^2 = 1$$

$$W\left(\begin{array}{c} \text{X} \\ \text{X} \end{array}\right)^2 + W\left(\begin{array}{c} \text{X} \\ \text{X} \end{array}\right)^2 = 1$$

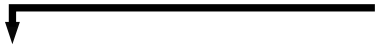

(a)

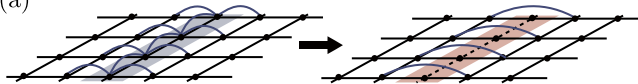

(b)

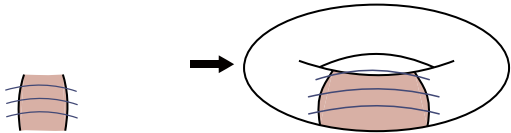

(c)

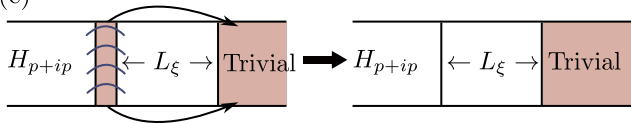

Supplement: Supplementary file 2 [file sm_symlocal.pdf]
