# Supplementary material for: Simulating 2D topological quantum phase transitions on a digital quantum computer
Source: arXiv:2312.05079 source file (2024-09-28)

(a)

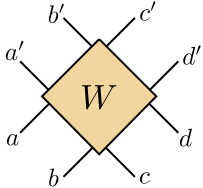

(b)

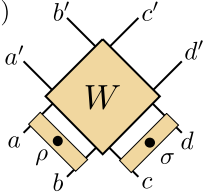

(c)

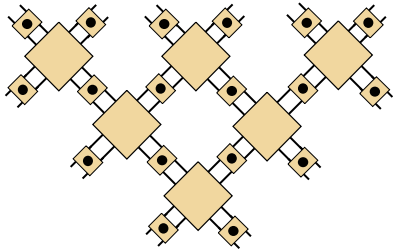



Lattice

Holographic

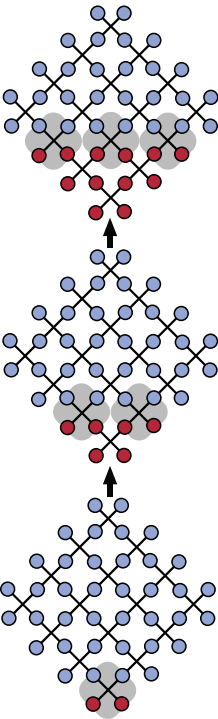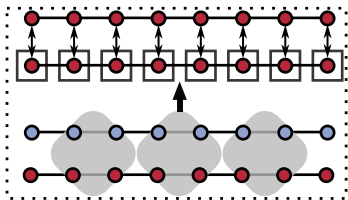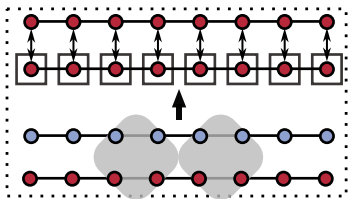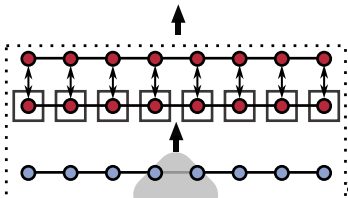

anc.

phys.

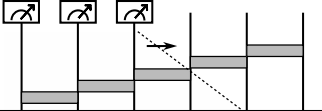

Supplement: Supplementary file 4 [file sm_tc_ds_V2.pdf]
